# Supplementary material for: Symmetry-resolved topology from interacting Green's functions
Source: arXiv:2511.22740 source file (2026-09-16)
Supplement: Supplementary file 1 [file supplement.tex]

% ****** Start of file apssamp.tex ******
%
%   This file is part of the APS files in the REVTeX 4.2 distribution.
%   Version 4.2a of REVTeX, December 2014
%
%   Copyright (c) 2014 The American Physical Society.
%
%   See the REVTeX 4 README file for restrictions and more information.
%
% TeX'ing this file requires that you have AMS-LaTeX 2.0 installed
% as well as the rest of the prerequisites for REVTeX 4.2
%
% See the REVTeX 4 README file
% It also requires running BibTeX. The commands are as follows:
%
%  1)  latex apssamp.tex
%  2)  bibtex apssamp
%  3)  latex apssamp.tex
%  4)  latex apssamp.tex
%
\documentclass[%
reprint,
onecolumn,
superscriptaddress,
%groupedaddress,
%unsortedaddress,
%runinaddress,
%frontmatterverbose, 
% preprint,
%preprintnumbers,
%nofootinbib,
%nobibnotes,
%bibnotes,
 amsmath,amssymb,
 aps,prb
%pra,
%prb,
%rmp,
%prstab,
%prstper,
%floatfix,
]{revtex4-2}

\usepackage[colorlinks=true,allcolors=blue]{hyperref}
\usepackage{cleveref}
\usepackage{graphicx}% Include figure files
\usepackage{dcolumn}% Align table columns on decimal point
\usepackage{bm}% bold math
\usepackage{xcolor}
\usepackage{xspace}

\newcommand{\gw}{\ensuremath{GW}\xspace}

\newcommand{\scgw}{sc$GW$\xspace}

\newcommand{\aSn}{$\alpha$-Sn\xspace}

% formatting

%\usepackage{hyperref}% add hypertext capabilities
%\usepackage[mathlines]{lineno}% Enable numbering of text and display math
%\linenumbers\relax % Commence numbering lines

%\usepackage[showframe,%Uncomment any one of the following lines to test 
%%scale=0.7, marginratio={1:1, 2:3}, ignoreall,% default settings
%%text={7in,10in},centering,
%%margin=1.5in,
%%total={6.5in,8.75in}, top=1.2in, left=0.9in, includefoot,
%%height=10in,a5paper,hmargin={3cm,0.8in},
%]{geometry}

\begin{document}

\title{Supplemental Information for ``Discovering topological phases in gray-Tin''}% using many-body Green's function methods}

\author{Gaurav Harsha}
\affiliation{Department of Chemistry, University of Michigan, Ann Arbor, MI 48109, USA}
\author{Selina Dirnb\"ock}
\affiliation{Department of Physics, University of Michigan, Ann Arbor, MI 48109, USA}
\affiliation{Institute of Solid State Physics, TU Wien, 1040 Vienna, Austria}
\author{Emanuel Gull}
\affiliation{Department of Physics, University of Michigan, Ann Arbor, MI 48109, USA}
\affiliation{Department of Physics, University of Warsaw, Pasteura 1, 02-093 Warsaw, Poland}
\author{Vojt\v{e}ch Vl\v{c}ek}
\affiliation{Department of Chemistry and Biochemistry, University of California, Santa Barbara, CA 93106, USA}
\affiliation{Department of Materials, University of California, Santa Barbara, CA 93106, USA}
\author{Dominika Zgid}%
\affiliation{Department of Chemistry, University of Michigan, Ann Arbor, MI 48109, USA}
\affiliation{Department of Physics, University of Michigan, Ann Arbor, MI 48109, USA}
\affiliation{Department of Physics, University of Warsaw, Pasteura 1, 02-093 Warsaw, Poland}
\date{\today}

\maketitle

\section{Orbital resolved band structures}
Figure 2 in the main manuscript presents the fully self-consistent \gw (\scgw) band structure and topological character of uniformly compressed \aSn for several lattice parameters.
The analysis is based on momentum-resolved occupations of symmetrized atomic orbitals (SAOs) along the $K$–$\Gamma$–$X$ high-symmetry path.
Here, we provide additional insight by comparing the orbital-resolved spectra of the valence $5s$ and $5p$ SAOs across different lattice constants.
To complement the results in the main text showing a transition from an inverted semimetal to a trivial insulator, Fig.~\ref{fig:orb_resolved_bands} displays the corresponding orbital-resolved spectra, highlighting the spectral weight from $5s$ and $5p$ SAOs.
A clear semimetal-to-insulator transition is observed, mediated by Dirac-like crossings around $a \simeq 6.55,\text{\AA}$ that originate primarily from the $5s$ bands.

\begin{figure}[h]
    \centering
    \includegraphics[width=0.98\linewidth]{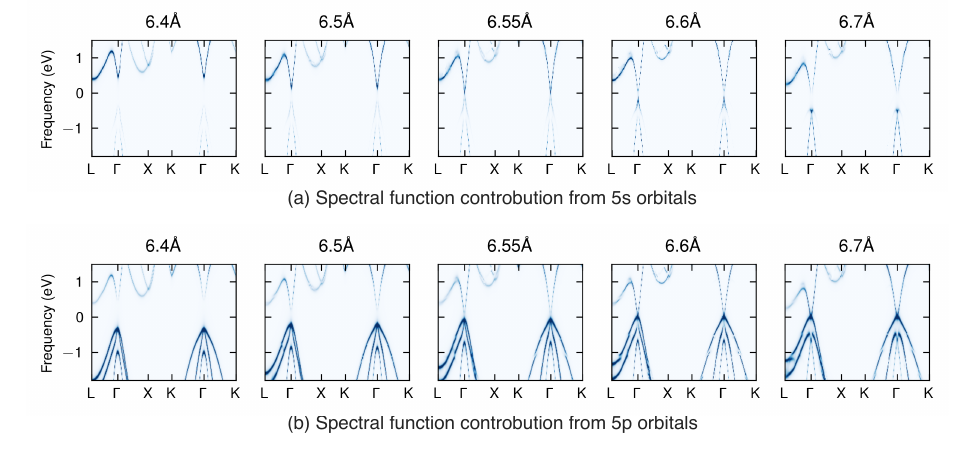}
    \caption{\textbf{Orbital resolved band structures of \aSn: } Contribution from (a) $5s$, and (b) $5p$ symmetrized atomic orbitals to the band structures of \aSn for various lattice constants.}
    \label{fig:orb_resolved_bands}
\end{figure}

\section{Orbital resolved band structures for in-plane strain along [111]}
Figure~\ref{fig:strain_111} shows the \scgw band structures of \aSn under compression along the [111] plane, using $a=6.7 \mathrm{\AA}$ as the reference geometry.
By comparing the contributions from $5s$ and $5p$ orbitals from panels (b) and (c), we see that that especially for 2\% compression, the $5s$-character conduction bands are nearly linear around $\Gamma$ at the Fermi level.
However, at $\Gamma$, both conduction and valence bands are dominated by $5p$ character, and a marginal lowering of the conduction band below the Fermi level leads to the formation of a Dirac semimetal.
Further compression opens the band gap, and destroys the band inversion, resulting in valence and conduction bands comprised purely of $5p$ and $5s$ characters, respectively.
This is also visible in orbital-resolved occupation trends shown in panel (d), as well as by comparing the 5\% strained geometry with results for $a=6.4 \, \mathrm{\AA}$ in Fig.~\ref{fig:orb_resolved_bands}.
Additionally, compressive strain along [111] destroys the M-shape which is related to topological surface states in \aSn, as noted in the main manuscript.

We note that a clear and obvious observation of Dirac band crossing in the [111] strained \aSn is nearly impossible beyond mean-field or tight-binding models, as the band crossing occurs within 100 meV around the Fermi level.
However, by decomposing the orbital contributions, we can amplify the signatures of such features.

\begin{figure}
    \centering
    \includegraphics[width=0.5\linewidth]{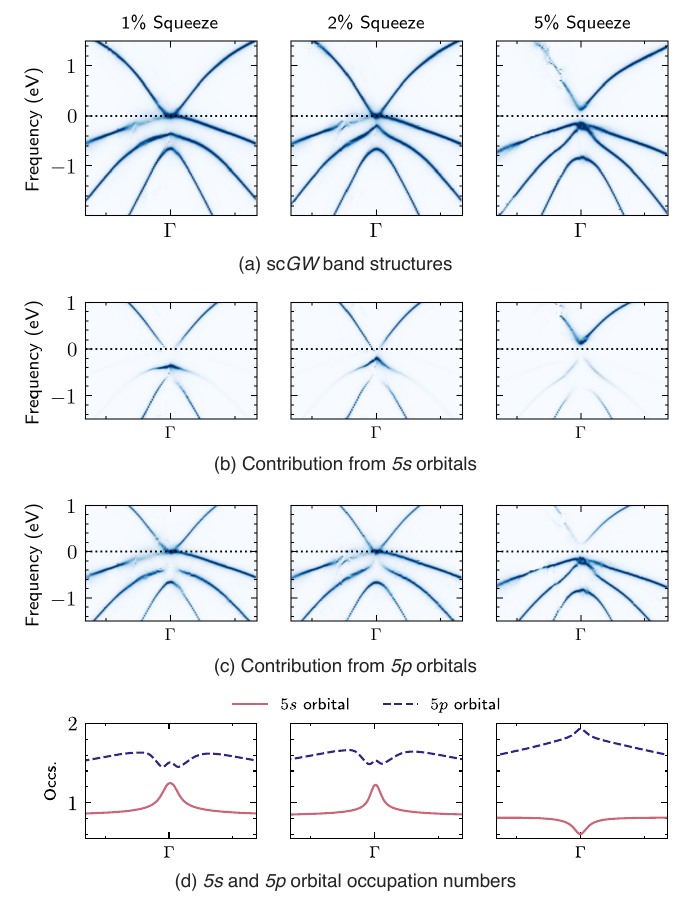}
    \caption{\textbf{Effect of in-plane compressive strain along [111] in bulk \aSn:} (a) \scgw band structure along the $P$-$\Gamma$-$X$ path; (b)-(c) spectral weight contribution from the $5s$ and $5p$ SAOs; and (d) corresponding orbital occupation trends. Compressive strain first introduces a marginal lowering of the conduction bands bands below the Fermi level, before eventually opening a trivial band-gap at $\Gamma$.} 
    \label{fig:strain_111}
\end{figure}

\begin{figure}[h]
    \centering
    \includegraphics[width=0.6\linewidth]{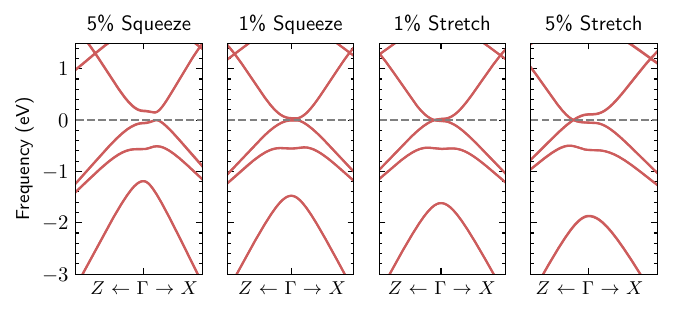}
    \caption{\textbf{Effect of [001] straining:} PBE bands for various degrees of compressive and tensile strain along the $c$-axis in \aSn. The results serve as a reference to compare the \scgw band structures in the main manuscript.}
    \label{fig:dft-001-bands}
\end{figure}

\section{PBE band structures for uniaxial strain along $c$-axis}
In the main manuscript, we analyze the effects of uniaxial straining along the $c$ axis, i.e., perpendicular to [001] plane, using the \scgw framework.
We show that while a tensile strain induces a topological Dirac semimetal phase, compressive strain results in a topological insulator (TI).
In addition to a non-trivial band gap around $\Gamma$, this TI phase exhibits a linearly-dispersing band crossing nearly 200 meV below the Fermi level.

Here, we show the results obtained from density functional theory to reiterate the efficacy of \scgw. 
Figure~\ref{fig:dft-001-bands} shows the PBE bands for the various $c$-axis strained \aSn lattices. For tensile strained configurations, PBE predicts a Dirac point along the $Z$-$\Gamma$ path, qualitatively consistent with \scgw.
For the squeezed configurations, while PBE predicts a band gap opening, it completely misses the peculiar band crossing just below the Fermi level, which is observed in the \gw results.
These results highlight the qualitative and quantitative prowess of \scgw over DFT.

\end{document}
